# Supplementary material for: To Do or Not to Do: Semantics and Patterns for Do Activities in UML PSSM State Machines
Source: arXiv:2309.14884 source file (2024-07-08)

|                             | RTC0  | SC0     | RTC1                                  | SC1                  | RTC2             | SC2                                 |                      | RTC3                                | SC3                        | RTC4                       | SC4                  |
|-----------------------------|-------|---------|---------------------------------------|----------------------|------------------|-------------------------------------|----------------------|-------------------------------------|----------------------------|----------------------------|----------------------|
| <b>event pool</b>           | -     | ()      | (turnOn)                              | ()                   | (measure)        | ()                                  | (gravityOk, refTemp) | (tempCompleted, CE(MeasureGravity)) | (tempCompleted)            | (tempCompleted)            | ()                   |
| <b>state configuration</b>  |       | Standby |                                       | Active{Wait1, Wait2} |                  | Active{MeasureTemp, MeasureGravity} |                      |                                     | Active{MeasureTemp, Wait2} |                            | Active{Wait1, Wait2} |
| <b>traversed transition</b> | $T_0$ |         | $T_{\text{turnOn}}, T_{1.0}, T_{2.0}$ |                      | $T_{m1}, T_{m2}$ |                                     |                      | $T_{2.CT}$                          |                            | $T_{\text{tempCompleted}}$ |                      |
| <b>do0</b>                  |       |         |                                       | prepareInst.         |                  |                                     |                      |                                     |                            |                            |                      |
| <b>do1</b>                  |       |         |                                       |                      |                  | measureTempAct                      |                      |                                     |                            |                            |                      |
| <b>do2</b>                  |       |         |                                       |                      |                  | measureGravity; ...                 |                      |                                     |                            |                            |                      |

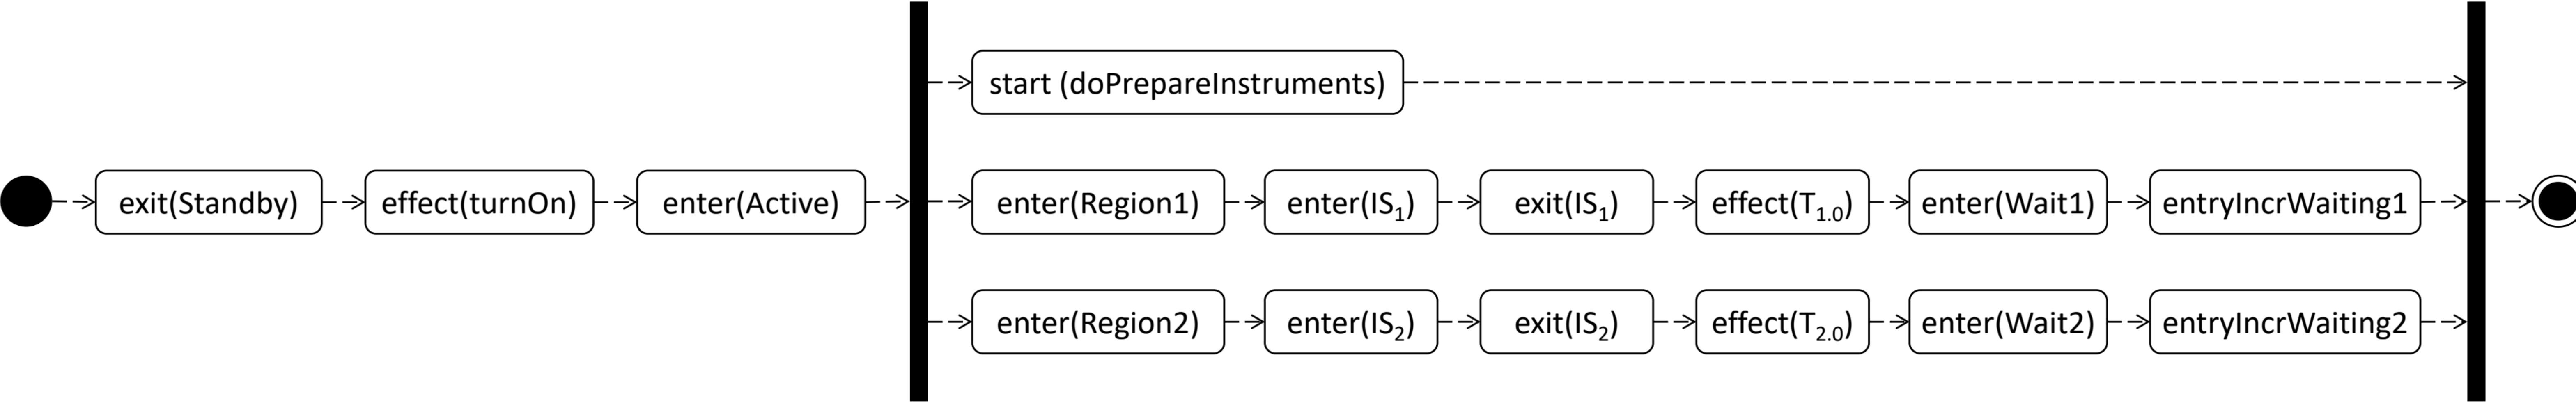

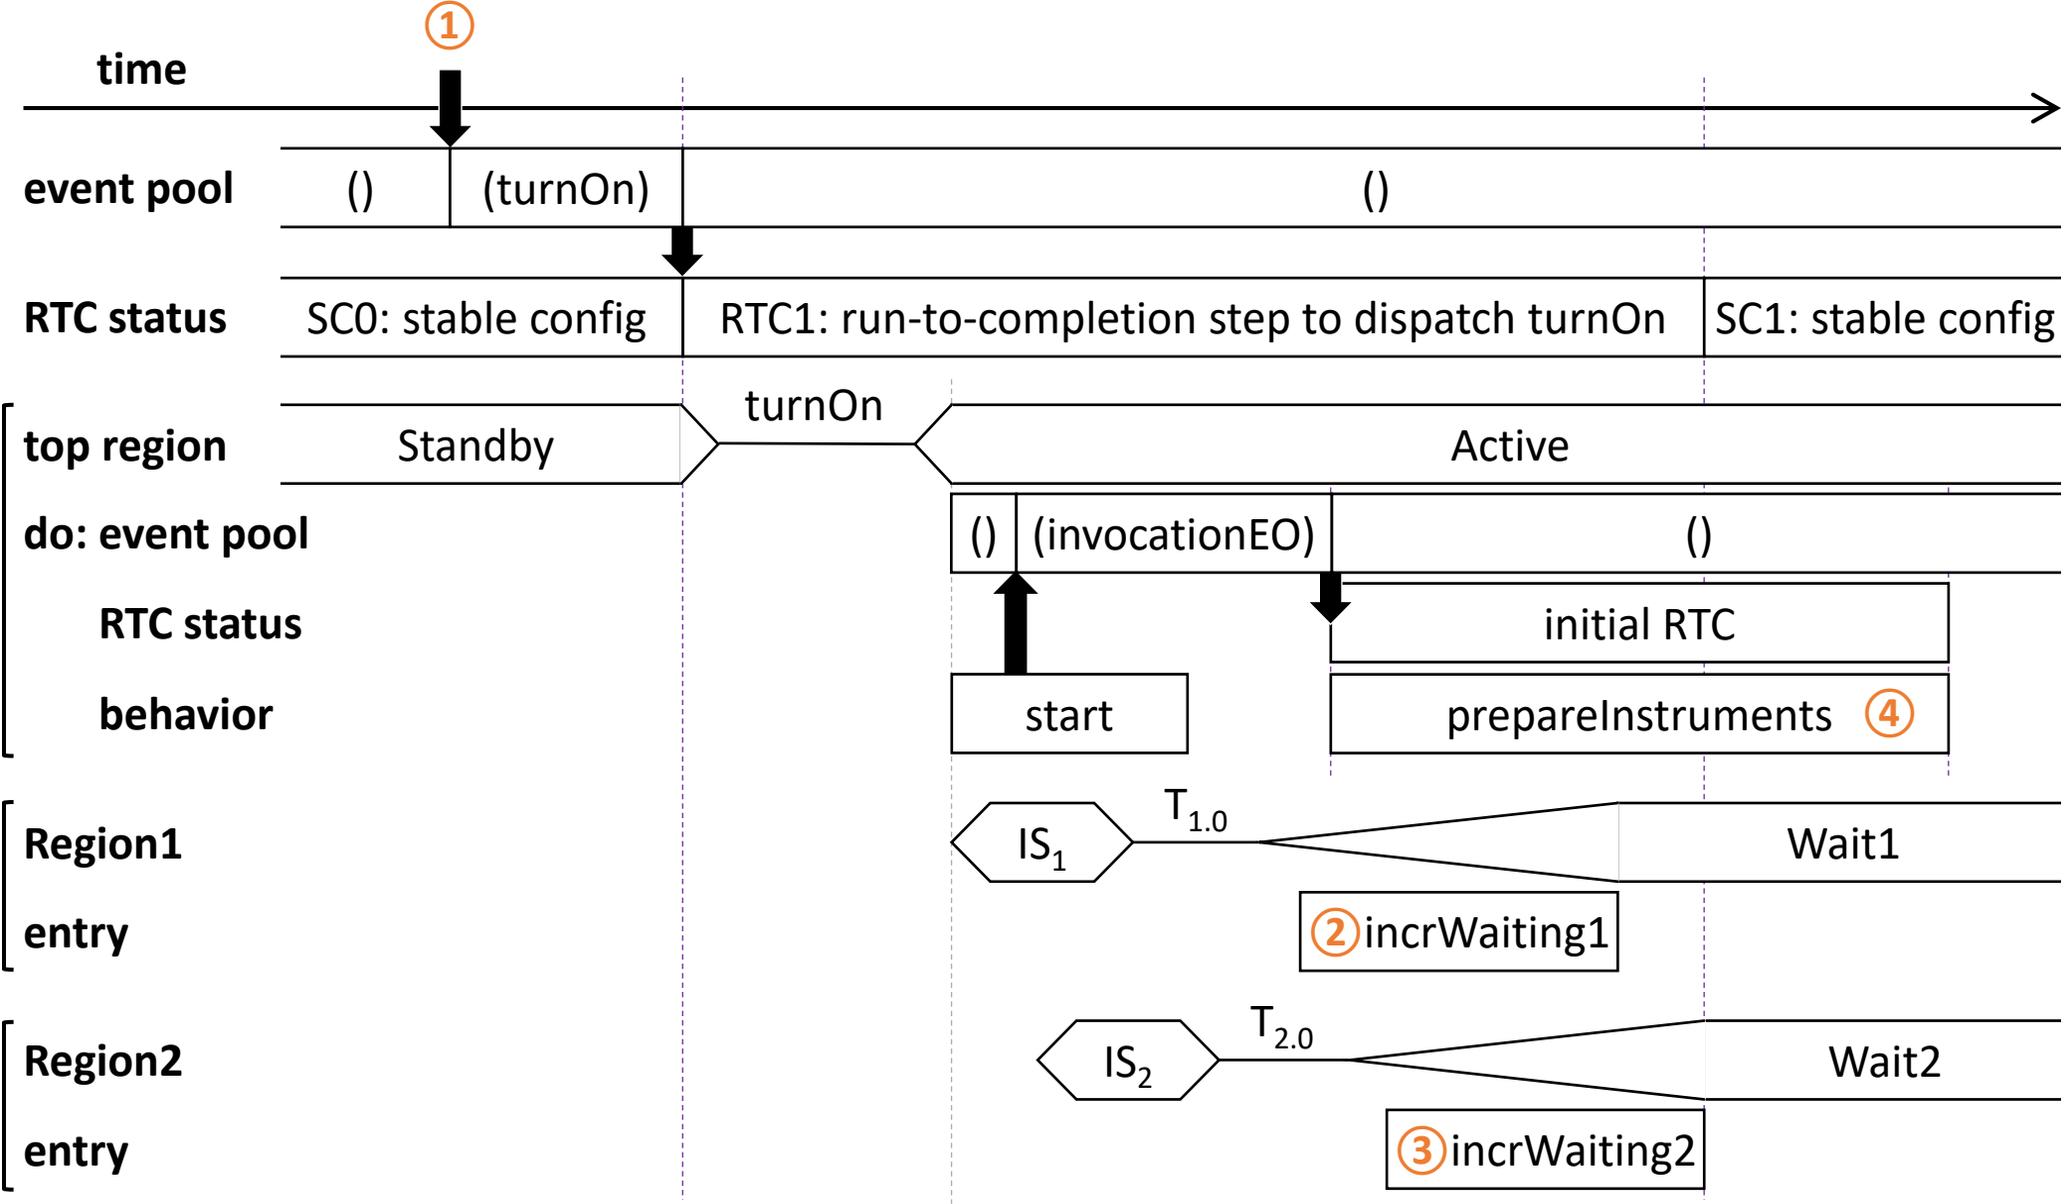

Supplement: Supplementary file 1 [file sm-micro-steps-crop.pdf]
